# Supplementary material for: Coactive-Staggered Feature in Weyl Materials for Enhancing the Anomalous Nernst Conductivity
Source: arXiv:2211.07773 ancillary file (2024-12-04)
Supplement: Supplementary file 1 [file Supplementary_Material.pdf]

# Supplemental Material: Coactive-Staggered Weyl Points Enhance the Anomalous Nernst Conductivity

Vsevolod Ivanov[1,2], Ella Banyas[2,3], and Liang Z. Tan[2]

[1]Accelerator Technology and Applied Physics Division, Lawrence Berkeley National Laboratory, Berkeley, CA 94720, USA
[2]Molecular Foundry, Lawrence Berkeley National Laboratory, Berkeley, CA 94720, USA
[3]Department of Physics, University of California, Berkeley, CA 94720, USA

## Supplementary Note 1: Additional Details on the calculation of Weyl metal $Rh_2NiSi$

Density functional theory calculations in VASP were performed on a $20\times20\times20\boldsymbol{k}$-point grid (4004 irreducible $\boldsymbol{k}$-points), with a convergence cutoff of $10^{-10}$, and 0.1eV smearing. Magnetic moments were fixed to the magnetic easy axis, and spin-orbit coupling was included. The cubic lattice parameter of 0% strain case was optimized with respect with system total energy. The epitaxial strains for the 1% and 2% cases were applied uniformly in the $x$-$y$ plane.

Wannierization was performed using the Wannier90 code using 36 bands, Rh and Ni $d$-orbitals, and Si $p$-orbitals, using a tollerance of $10^{-10}$. Disentanglement was done in a 3eV window surrounding $E_F$, using a tolerance of $10^{-11}$.

For each of the strain cases, the tight-binding model computed with Wannier90 was used as input in WannierTools to compute the AHC and ANC. The custom module for computing the ANC is identical to the one for computing AHC in the native WannierTools code, but uses a special weight function (Eq. 5 in the main text), instead of the Fermi factor. Calculations were performed on a $201\times201\times201$ $k$-point grid at 100K.

Nodes were found using a two step process, first by running the "FindNodes" module to locate degeneracies, and then the "WeylChirality" module was run on the degeneracies to confirm their topological nature. Bands 28-35 were searched for Weyl points to capture a complete window with $\pm0.5$ eV of the Fermi level.

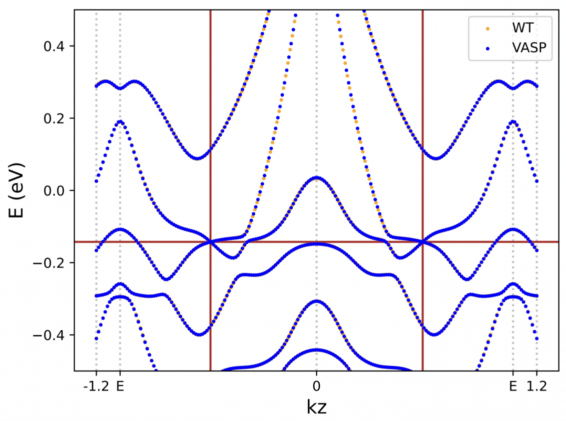


Figure S1: Example Weyl node from one of the strain cases of $Rh_2NiSi$. There a clear crossing in the dispersion at the exact energy and momentum space location of the Weyl node, both in the DFT and Wannierized bands.

In order to track Weyl points between different strain cases, nodes are first sorted into symmetry-related sets. To do this, we start off by only keeping nodes with $|k_z| > 0.01$, or equivalently, pairs with a separation

Table S1: Symmetry-inequivalent Weyl points in (unstrained) $Rh_2NiSi$ with their Cartesian locations in units of $2\pi/a$ and their energies in eV.

| $(\lvert k_x \rvert, \lvert k_y \rvert, \lvert k_z \rvert)$ | Energy |
|---|---|
| $(0.0023, 0.9474, 0.1320)$ | $-0.4989$ |
| $(0.6483, 0.6501, 0.0239)$ | $-0.3559$ |
| $(0.0001, 0.8658, 0.5453)$ | $-0.3061$ |
| $(0.3177, 0.3188, 0.6312)$ | $-0.2630$ |
| $(0.0003, 0.7505, 0.4304)$ | $-0.2592$ |
| $(0.4723, 0.7476, 0.1679)$ | $-0.2560$ |
| $(0.0013, 0.4794, 0.7502)$ | $-0.2017$ |
| $(0.0008, 0.5427, 0.7807)$ | $-0.1955$ |
| $(0.6118, 0.6119, 0.2281)$ | $-0.1510$ |
| $(0.0003, 0.0019, 0.6019)$ | $-0.1234$ |
| $(0.0001, 0.7646, 0.5913)$ | $-0.1080$ |
| $(0.1629, 0.5473, 0.1630)$ | $-0.0688$ |
| $(0.0002, 0.9996, 0.0924)$ | $-0.0638$ |
| $(0.0066, 0.0068, 0.8472)$ | $-0.0600$ |
| $(0.0003, 0.8309, 0.0768)$ | $0.0278$ |
| $(0.0283, 0.6514, 0.6276)$ | $0.0494$ |
| $(0.0180, 0.6527, 0.6284)$ | $0.0520$ |
| $(0.0013, 0.6327, 0.6195)$ | $0.0658$ |
| $(0.0001, 0.1844, 0.8852)$ | $0.0861$ |
| $(0.0002, 0.0008, 0.9252)$ | $0.0956$ |
| $(0.0000, 0.0003, 0.9167)$ | $0.0971$ |
| $(0.0226, 0.0325, 0.2955)$ | $0.1378$ |

greather than approximately a hundredth of the BZ, since small z-separations will contribute only minimally to the AHC. Nodes were sorted into sets with the same $|k_z|$, energy, and xy $\boldsymbol{k}$-coordinates that were related by the symmetry transformations of the space group.

Then, finally, we combined the sorted nodes from the three strain cases and tracked symmetry-unique nodes across strain. Note that we are neglecting node pairs that are created or annihilated by strain. We tracked nodes by requiring monotonic changes in the energy and $k_z$-value with strain, and by matching nodes to those with the smallest k-displacement first, and confirming that their chiralities matched as well. There were 22 nodes that could be fully tracked between all strain cases, which are listed in Table S1. It was confirmed that all identified Weyl points correspond to nodes by finding them in both the DFT and Wannier-interpolated band structures, as shown in Figure S1.

## Supplementary Note 2: Additional Details on the Creation of CS Weyls in Dirac Semimetals

Here we explore several approaches to creating CS Weyl point configurations from a Dirac semimetal. Dirac semimetals are materials possessing both time-reversal ($\mathcal{T}$) and inversion ($\mathcal{I}$) symmetries, which host a four-fold degeneracy with linear dispersion called a Dirac point [S1, S27]. Excitations near this point can be described by the four-fold Hamiltonian of a Dirac fermion, which in turn can be decomposed into a pair of $2 \times 2$ Hamiltonians describing Weyl fermions [S22, S23] of opposite chirality. If the $\mathcal{T}$ and/or $\mathcal{I}$ symmetries are broken, the degeneracy of the Dirac point is also broken, splitting it into equal numbers of positive and negative chirality Weyl points [S28, S8, S4]. Breaking time-reversal symmetry in a Dirac semimetal can be used to create coactive-staggered arrangements of Weyl points, as discussed in the main text. Experimental symmetry-breaking techniques include introducing an external magnetic field [S5], doping with magnetic atoms [S7, S2], or creating a layered heterostructure consisting of the Dirac semimetal and a magnetic insulator [S6].

The procedure for creating a coactive staggered configuration of Weyl points in a Dirac semimetal can be understood through a simple $k \cdot p$ model. We start with a simple four band tight binding model [S19, S16]

$$\mathcal{H} = \begin{bmatrix} \mathcal{M}^{\mathcal{A}} + \Delta\sigma_z & \mathcal{P} \\ \mathcal{P} & \mathcal{M}^{\mathcal{B}} - \Delta\sigma_z \end{bmatrix}, \tag{S1}$$

where $\mathcal{M}^{\lambda} = M_0^{\lambda} + 6M_1^{\lambda} - 2M_1^{\lambda}(\cos k_x + \cos k_y + \cos k_z)$ defines the bands, while the off diagonal term $\mathcal{P} = \sum_{i=xyz} P_i \sin k_i \sigma_i$ breaks the symmetry of the bands. The magnetic term $\Delta\sigma_z$ introduces a Zeeman splitting, and throughout, we are using the Pauli matrices $\boldsymbol{\sigma} = (\sigma_x, \sigma_y, \sigma_z)$. For the purpose of analyzing this Hamiltonian, in the subsequent discussion, we take the parameters to be $M_0^A = M_0^B = 0$, $M_1^A = -M_1^B = M$, $P_z = 0$, and $P_x = P_y = 1$.

Neglecting $\mathcal{P}$ and expanding the Hamiltonian around the $\Gamma$-point to second order we find $\mathcal{M}^{\lambda} \approx M_0^{\lambda} + M_1^{\lambda}(k_x^2 + k_y^2 + k_z^2)$, giving two doubly degenerate parabolic bands that cross along the $k_z$-axis. Diagonalizng the Hamiltonian, we obtain the exact form of the bands along the $k_z$-axis: $\pm(1-2M-\Delta+2M\cos k_z)$, which in the absence of Zeeman splitting $\Delta = 0$, form 4-fold degenerate crossings at $k_z = \pm\arccos(1 - 1/2A)$. As $\Delta$ is increased, the two 4-fold degenerate crossings split into four pairs of Weyl points, two located at the Fermi level , and the other two pairs positioned above and below $E_F$. Elsewhere in the Brillouin zone, the Hamiltonian is gapped. Here already we have already obtained a coactive-staggered Weyl point configuration; for small $\Delta$, the Berry curvature contributions of the two pairs of Weyl points at $E_F$ are nearly cancelling, while the pairs of Weyls above and below $E_F$ generate fields of Berry curvature flux in opposite directions, due to their oppositely oriented chiralities. This would in turn result in peaks of opposite sign in the AHC, and an enhancement of the peak in the ANC at the Fermi energy.

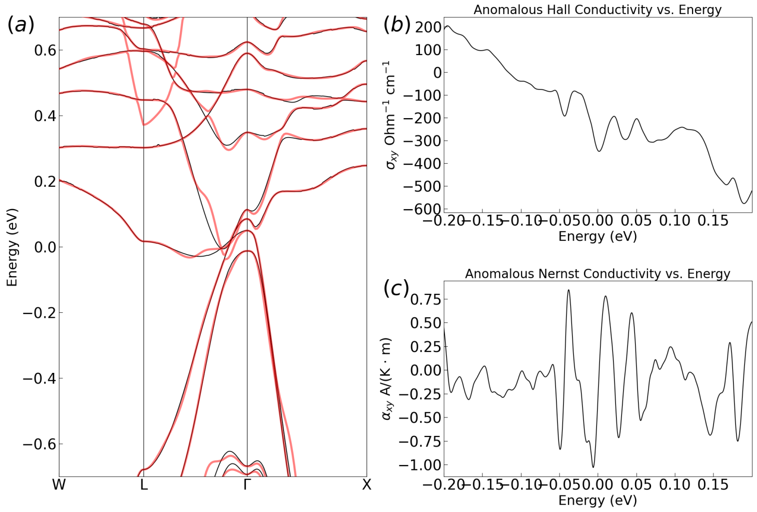


Figure S2: Electronic structure and transport properties of GdPtBi. Bandstructure, and Wannier fit in red (a), as well as anomalous Hall (b) and Nernst (c) conductivities at 20K.

In order to investigate the realization of coactive-staggered Weyl configurations using various approaches in real materials, we perform first principles electronic structure calculations on GdPtBi (ferromagnetic spin alignment using external magnetic field), $Ba_0.5Eu_0.5AgBi$ (introducing magnetism through substitutional

doping), and a structure composed of alternating layers of $PdTe_2$ and $VI_2$ (heterostructure of magnetic insulator and Dirac materials). Calculations were performed with the Wien2k code [S3] with spin orbit coupling included, using the experimental lattice parameters and the atom positions obtained through structural relaxation. Calculations for $Ba_0.5Eu_0.5AgBi$ used the modified Becke-Johnson exchange correlation potential [S21], while the others used PBE functionals [S17]. In order to compute anomalous Hall and Nernst conductivities, projection onto maximally localized Wannier functions was performed using the wien2wannier utility and Wannier90 [S11, S15, S18]. The Wannier tight-binding Hamiltonians were then used to compute the anomalous Hall conductivity using WannierTools [S25] at 20K, as well as the anomalous Nernst conductivity at 20K using a modified version of WannierTools developed by one of us.

First we will cover the creation of coactive-staggered Weyl points in a Dirac material using an external magnetic field, by considering the case of GdPtBi. The half-Heusler GdPtBi is antiferromagnetic below $T_N = 9$K [S20], and hosts an enforced four-fold degeneracy at the Γ-point composed of four Bi $6p$ bands $|j, m_j\rangle = |3/2, \pm 1/2\rangle, |3/2, \pm 3/2\rangle$, which is enforced due to the $T_d$ symmetry of the crystal [S9]. Under an applied magnetic field, time reversal symmetry is broken and the degeneracy is lifted, creating a number of Weyl points [S5]. For a large enough external field, the Gd spins would completely align ferromagnetically, which is the option we explore, computing the electronic structure of ferromagnetic GdPtBi (Figure S2). we find a quite small value for the AHC at $E_F$, peaking at $\sim 340\ \Omega^{-1}\ \text{cm}^{-1}$, though the experimentally measured value of $60\ \Omega^{-1}\ \text{cm}^{-1}$ is even smaller. This is expected due to the low density of states at the Fermi energy, and the discrepancy in magnitude is likely due to the magnetic field that would be needed to completely align all of the Gd spins ferromagnetically being much larger than what is acheivable experimentally. The plot of the AHC as a function of energy shown in **??**b, exhibits the characteristic two peak structure of a coactive-staggered Weyl configuration around the Fermi energy. However, this signal is dominated by a large background of negative AHC stemming from the Berry curvature contribution from other bands. Due to the small magntitude of the AHC, and the coactive-staggered Weyl contribution being small compared to other sources of Berry curvature in the Brillouin zone, the ANC signal is quite weak (Figure S2c), with the peak value of $\sim -1$ A/K·m barely exceeding the magnitudes of the nearby fluctuations.

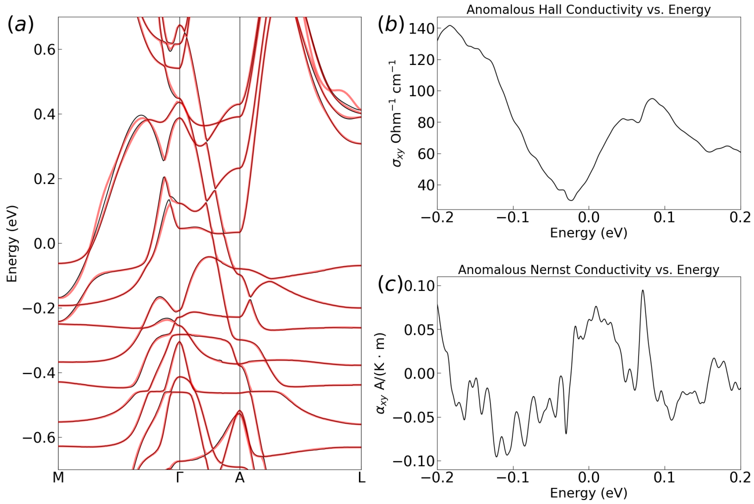


Figure S3: Electronic structure and transport properties of $Ba_{0.5}Eu_{0.5}AgBi$. Bandstructure, and Wannier fit in red (a), as well as anomalous Hall (b) and Nernst (c) conductivities at 20K.

Another possibility is to introduce magnetism into a Dirac system through doping with a magnetic element. The hexagonal BaXBi compounds (where X = Ag, Au, or Cu) host a Dirac node along the $\Gamma - A$ high symmetry line in the Brillouin zone [S7]. In particular for BaAgBi, calculations predict that there are no other bands crossing the Fermi energy, thus the electron filling pins the Dirac node exactly at $E_F$. For this material, Ba can be continuously replaced by Eu without affecting the crystal structure, which makes the material ferromagnetic due to the Eu magnetic moments. The simplest doping scenario is at half-substitution, $Ba_{0.5}Eu_{0.5}AgBi$, which can be considered stoichiometrically using a doubled unit cell with one atom of Ba and on atom of Eu. For this doping, the ferromagnetic order breaks time-reversal symmetry and splits the Dirac cone into several Weyl points very close to the Fermi energy, making a nearly ideal Weyl semimetal candidate with few trivial bands [S7]. However, more recent calculations [S2], have suggested that a number of other bands cross the Fermi energy, and suggest that the Dirac node splits into four Weyl points, which should form a coactive-staggered configuration. Our calculations (Figure S3) indeed reveal

that the Weyl crossings near $E_F$ which arise from the Dirac node, along with several trivial bands which cross the Fermi level. The AHC shown in Figure S3b indeed shows a coactive-staggered Weyl configuration, but just as the case with GdPtBi, the contribution is small, and is overshadowed by the background signal, which results in only a small peak in the ANC (Figure S3c).

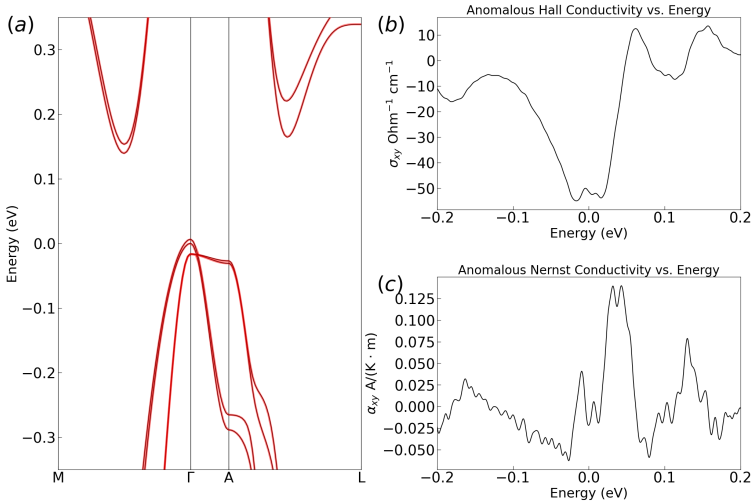


Figure S4: Electronic structure and transport properties of $PdTe_2$-$VI_2$ heterostructure. Bandstructure, and Wannier fit in red (a), as well as anomalous Hall (b) and Nernst (c) conductivities at 20K.

To demonstrate a potential heterostructure hosting a CS configuration of Weyl points, candidate Dirac semimetals and magnetic insulators from the class of transition-metal dichalcogenides (TMDC) were considered. TMDCs are multifunctional materials possessing a number of interesting phases, including charge density wave, superconductivity, and topological phases, and can be used in the construction of Van der Waals heterostructures [S13, S12]. To test this concept, we simulate a heterostructure of $PdTe_2$ and $VI_2$ monolayers, which have less than a 1% lattice mismatch [S10, S26]. $PdTe_2$ is a Dirac metal, with a Dirac cone along the $\Gamma - A$ direction [S26], while bulk $VI_2$ is an insulator that undergoes successive transitions through antiferromagnetic orders at $T_N = 16.3$K and $T_N = 15$K [S10]. Theoretical calculations show that monolayer $VI_2$ is also insulating and appears to favor Neel 120° in-plane antiferromagnetic order [S24]. However, the details of the magnetic order of bulk and monolayer $VI_2$ are not settled [S14]. We perform calculations on a heterostructure of $PdTe_2$ and $VI_2$ monolayers magnetically ordered along the $\langle 001 \rangle$ direction. Just as before, the four-fold Dirac crossing is split due to the broken time reversal symmetry into Weyl crossings near the Fermi energy (Figure S4. However, the separation between the Weyl points is extremely small, and would likely be washed out by temperature broadening effects in an experimental realization of this heterostructure. Once again, while a coactive-staggered Weyl configuration is generated, the small separation of the Weyl points leads to a very small value of the AHC and ANC signals. It should also be noted that such a heterostructure approach has an inherent limitation – the Dirac point lies on the $k_z$ axis and stacking the layers in the $z$-direction leads to a folding of the Brillouin zone along the $k_z$-direction, which ultimately limits the possible separation of Weyl nodes and the magnitude of the AHC/ANC. A more generalized approach would have to involve a systematic search for lattice-compatible materials where the stacking direction doesn't interfere w/ the splitting.

It is clear from the preceding examples that the approach of creating CS Weyl configurations starting from a Dirac semimetal has a number of limitations. Firstly, Dirac semimetals tend to have a low density of states at the Fermi level, on which transport properties are highly dependent. Secondly, the magnetism in these systems results in a relatively small separation of the Weyl points both in energy and momentum space. While a small energy separation can be favorable for tuning the ANC, the magnitude of the AHC (and therefore the ANC) is proportional to the momentum-space separation of the Weyl points. In order to achieve a large ANC, either the bands generating the Weyl points must be flat, resulting in a large density of states and momentum-space separation, or the overall number of Weyl pairs must be very large in order to compensate for the small contribution of each individual pair.

## Supplementary Note 3: Derivation of the upper bound for the anomalous Nernst coefficient

We seek to maximize the anomalous Nernst coefficient

$$\alpha(T,\mu) = -\frac{1}{eT}\int w\left(\frac{\epsilon-\mu}{k_B T}\right)\sigma(T=0,\epsilon)d\epsilon, \tag{S2}$$

given the constraint

$$\bar{\sigma}^2 = \int \sigma^2(T=0,\epsilon)d\epsilon, \tag{S3}$$

that sets the size $\bar{\sigma}$ of the anomalous Hall effect in the material, which itself depends on the quantity and distribution of Berry curvature sources in the Brillouin zone. The Euler-Lagrange equation for this constraint problem is

$$\frac{\partial w\sigma}{\partial \sigma} - \cancelto{0}{\frac{d}{d\epsilon}\frac{\partial w}{\partial \sigma'}} + \lambda\left(\frac{\partial \sigma^2}{\sigma} + \cancelto{0}{\frac{d}{d\epsilon}\frac{\partial \sigma^2}{\partial \sigma}}\right) = 0, \tag{S4}$$

giving $\sigma_{\text{opt}}(0,\epsilon) = -w((\epsilon-\mu)/k_BT)/2\lambda$, which can also be obtained by inspection of equations S2 and S3. This function has a positive peak just aboe and a negative peak just below $\mu$, precisely having the shape of the coactive-staggered configuration discussed in the text. The factor $\lambda$ can be found from Eq. S3:

$$\bar{\sigma}^2 = \frac{1}{4\lambda^2}\int w^2\left(\frac{\epsilon-\mu}{k_BT}\right)d\epsilon = \frac{k_BT}{4\lambda^2}\int w^2(x)dx = \frac{k_BT}{4\lambda^2}\frac{\pi^2-6}{18} \tag{S5}$$
$$\rightarrow \lambda = \frac{1}{6\bar{\sigma}}\sqrt{\frac{\pi^2-6}{2}k_BT}.$$

The separation of the two peaks in the optimal anomalous Hall coefficient $\sigma_{\text{opt}}$, can be found by taking the derivative of the weight function $w(x)$, obtaining $\Delta E = 3.0868 k_B T$.

Now we can obtain an upper bound $\alpha_{\max}$ for the anomalous Nernst coefficient for a given size of the anomalous Hall $s\bar{i}gma$ and peak separation $\Delta E$. We have

$$\alpha_{\max} = \frac{1}{eT}\frac{1}{2\lambda}\int w^2\left(\frac{\epsilon-\mu}{k_BT}\right)d\epsilon = C\frac{k_B}{e}\bar{\sigma}\Delta E^{-\frac{1}{2}}, \tag{S6}$$

Where $C$ is a constant,

$$C = \sqrt{3.0868\frac{\pi^2-6}{18}} \approx 0.814614 \tag{S7}$$

## References


[S1] N. P. Armitage, E. J. Mele, and Ashvin Vishwanath. Weyl and dirac semimetals in three-dimensional solids. *Rev. Mod. Phys.*, 90:015001, Jan 2018.

[S2] Chanchal K. Barman, Chiranjit Mondal, Biswarup Pathak, and Aftab Alam. Symmetry-driven topological phases in $x$AgBi$(x = \mathrm{Ba}, \mathrm{Sr})$: An ab initio hybrid functional calculation. *Phys. Rev. Materials*, 4:084201, Aug 2020.

[S3] Peter Blaha, Karlheinz Schwarz, Fabien Tran, Robert Laskowski, Georg K. H. Madsen, and Laurence D. Marks. Wien2k: An apw+lo program for calculating the properties of solids. *The Journal of Chemical Physics*, 152(7):074101, 2020.

[S4] A. A. Burkov and Leon Balents. Weyl semimetal in a topological insulator multilayer. *Phys. Rev. Lett.*, 107:127205, Sep 2011.

[S5] Jennifer Cano, Barry Bradlyn, Zhijun Wang, Max Hirschberger, N. P. Ong, and B. A. Bernevig. Chiral anomaly factory: Creating weyl fermions with a magnetic field. *Phys. Rev. B*, 95:161306, Apr 2017.

[S6] Cui-Zu Chang. Marriage of topology and magnetism. *Nature Materials*, 19(5):484–485, May 2020.

[S7] Yongping Du, Bo Wan, Di Wang, Li Sheng, Chun-Gang Duan, and Xiangang Wan. Dirac and weyl semimetal in xybi (x = ba, eu; y = cu, ag and au). *Scientific Reports*, 5(1):14423, Sep 2015.

[S8] Gábor B. Halász and Leon Balents. Time-reversal invariant realization of the weyl semimetal phase. *Phys. Rev. B*, 85:035103, Jan 2012.

[S9] Max Hirschberger, Satya Kushwaha, Zhijun Wang, Quinn Gibson, Sihang Liang, Carina A. Belvin, B. A. Bernevig, R. J. Cava, and N. P. Ong. The chiral anomaly and thermopower of weyl fermions in the half-heusler gdptbi. *Nature Materials*, 15(11):1161–1165, Nov 2016.

[S10] S.R. Kuindersma, C. Haas, J.P. Sanchez, and R. Al. Magnetic structures and properties of vi2. *Solid State Communications*, 30(6):403–408, 1979.

[S11] Jan Kuneš, Ryotaro Arita, Philipp Wissgott, Alessandro Toschi, Hiroaki Ikeda, and Karsten Held. Wien2wannier: From linearized augmented plane waves to maximally localized wannier functions. *Computer Physics Communications*, 181(11):1888–1895, 2010.

[S12] Yuan Liu, Nathan O. Weiss, Xidong Duan, Hung-Chieh Cheng, Yu Huang, and Xiangfeng Duan. Van der waals heterostructures and devices. *Nature Reviews Materials*, 1(9):16042, Jul 2016.

[S13] Sajedeh Manzeli, Dmitry Ovchinnikov, Diego Pasquier, Oleg V. Yazyev, and Andras Kis. 2d transition metal dichalcogenides. *Nature Reviews Materials*, 2(8):17033, Jun 2017.

[S14] Michael A. McGuire. Crystal and magnetic structures in layered, transition metal dihalides and trihalides. *Crystals*, 7(5), 4 2017.

[S15] Arash A. Mostofi, Jonathan R. Yates, Young-Su Lee, Ivo Souza, David Vanderbilt, and Nicola Marzari. wannier90: A tool for obtaining maximally-localised wannier functions. *Computer Physics Communications*, 178(9):685–699, 2008.

[S16] Jonathan Noky, Johannes Gooth, Claudia Felser, and Yan Sun. Characterization of topological band structures away from the fermi level by the anomalous nernst effect. *Phys. Rev. B*, 98:241106, Dec 2018.

[S17] John P. Perdew, Kieron Burke, and Matthias Ernzerhof. Generalized gradient approximation made simple. *Phys. Rev. Lett.*, 77:3865–3868, Oct 1996.

[S18] Giovanni Pizzi, Valerio Vitale, Ryotaro Arita, Stefan Blügel, Frank Freimuth, Guillaume Géranton, Marco Gibertini, Dominik Gresch, Charles Johnson, Takashi Koretsune, Julen Ibañez-Azpiroz, Hyungjun Lee, Jae-Mo Lihm, Daniel Marchand, Antimo Marrazzo, Yuriy Mokrousov, Jamal I Mustafa, Yoshiro Nohara, Yusuke Nomura, Lorenzo Paulatto, Samuel Poncé, Thomas Ponweiser, Junfeng Qiao, Florian Thöle, Stepan S Tsirkin, Małgorzata Wierzbowska, Nicola Marzari, David Vanderbilt, Ivo Souza, Arash A Mostofi, and Jonathan R Yates. Wannier90 as a community code: new features and applications. *Journal of Physics: Condensed Matter*, 32(16):165902, jan 2020.

[S19] Tomá š Rauch, Huong Nguyen Minh, Jürgen Henk, and Ingrid Mertig. Model for ferromagnetic weyl and nodal line semimetals: Topological invariants, surface states, anomalous and spin hall effect. *Phys. Rev. B*, 96:235103, Dec 2017.

[S20] Chandra Shekhar, Nitesh Kumar, V. Grinenko, Sanjay Singh, R. Sarkar, H. Luetkens, Shu-Chun Wu, Yang Zhang, Alexander C. Komarek, Erik Kampert, Yurii Skourski, Jochen Wosnitza, Walter Schnelle, Alix McCollam, Uli Zeitler, Jürgen Kübler, Binghai Yan, H.-H. Klauss, S. S. P. Parkin, and C. Felser. Anomalous hall effect in weyl semimetal half-heusler compounds rptbi (r = gd and nd). *Proceedings of the National Academy of Sciences*, 115(37):9140–9144, 2018.

[S21] Fabien Tran and Peter Blaha. Accurate band gaps of semiconductors and insulators with a semilocal exchange-correlation potential. *Phys. Rev. Lett.*, 102:226401, Jun 2009.

[S22] G. E. Volovik. Zeros in the fermion spectrum in superfluid systems as diabolical points. *JETP Letters*, 46:81, 1987.

[S23] Xiangang Wan, Ari M. Turner, Ashvin Vishwanath, and Sergey Y. Savrasov. Topological semimetal and fermi-arc surface states in the electronic structure of pyrochlore iridates. *Phys. Rev. B*, 83:205101, May 2011.

[S24] A H M Abdul Wasey, Debjani Karmakar, and G P Das. Manifestation of long-range ordered state in layered $vx_2$ (x = cl, br, i) systems. *Journal of Physics: Condensed Matter*, 25(47):476001, oct 2013.

[S25] QuanSheng Wu, ShengNan Zhang, Hai-Feng Song, Matthias Troyer, and Alexey A. Soluyanov. Wanniertools : An open-source software package for novel topological materials. *Computer Physics Communications*, 224:405 – 416, 2018.

[S26] R. C. Xiao, P. L. Gong, Q. S. Wu, W. J. Lu, M. J. Wei, J. Y. Li, H. Y. Lv, X. Luo, P. Tong, X. B. Zhu, and Y. P. Sun. Manipulation of type-i and type-ii dirac points in $pdte_2$ superconductor by external pressure. *Phys. Rev. B*, 96:075101, Aug 2017.

[S27] S. M. Young, S. Zaheer, J. C. Y. Teo, C. L. Kane, E. J. Mele, and A. M. Rappe. Dirac semimetal in three dimensions. *Phys. Rev. Lett.*, 108:140405, Apr 2012.

[S28] A. A. Zyuzin, Si Wu, and A. A. Burkov. Weyl semimetal with broken time reversal and inversion symmetries. *Phys. Rev. B*, 85:165110, Apr 2012.
